# Supplementary material for: Social Media Identity Deception Detection: A Survey
Source: arXiv:2103.04673 ancillary file (2021-04-22)
Supplement: Supplementary file 1 [file Social_Media_Identity_Deception__arXiv.pdf]

# Online Appendix to: Social Media Identity Deception Detection: A Survey

AHMED ALHARBI, HAI DONG, XUN YI, ZAHIR TARI, and IBRAHIM KHALIL, School of Computing Technologies, RMIT University, Australia

**ACM Reference Format:**
Ahmed Alharbi, Hai Dong, Xun Yi, Zahir Tari, and Ibrahim Khalil. 2021. Online Appendix to: Social Media Identity Deception Detection: A Survey. *ACM Comput. Surv.* 37, 4, Article 111 (January 2021), 13 pages. https://doi.org/10.1145/1122445.1122456

Authors' address: Ahmed Alharbi, ahmed.alharbi@rmit.edu.au; Hai Dong, hai.dong@rmit.edu.au; Xun Yi, xun.yi@rmit.edu.au; Zahir Tari, zahir.tari@rmit.edu.au; Ibrahim Khalil, ibrahim.khalil@rmit.edu.au, School of Computing Technologies, RMIT University, Melbourne, Australia.

Permission to make digital or hard copies of all or part of this work for personal or classroom use is granted without fee provided that copies are not made or distributed for profit or commercial advantage and that copies bear this notice and the full citation on the first page. Copyrights for components of this work owned by others than ACM must be honored. Abstracting with credit is permitted. To copy otherwise, or republish, to post on servers or to redistribute to lists, requires prior specific permission and/or a fee. Request permissions from permissions@acm.org.
© 2021 Association for Computing Machinery.
0360-0300/2021/1-ART111 $15.00
https://doi.org/10.1145/1122445.1122456

# APPENDIX

Table 1. Existing works on Sybil detection techniques

| Ref | Year | Social media | Goal | Technique | Features | Datasets |
|---|---|---|---|---|---|---|
| [40] | 2017 | Generic | Detection of Sybil | Integrate labels and social network structure<br>Define badness score for nodes using random walk<br>Develop an iterative algorithm | Label-augmented social network | **Facebook:** 4,039 nodes and 88,234 edges<br>**Twitter:** 41,652,230 nodes and 1,202,513,046 edges<br>**Enron:** 33,696 nodes and 180,811 edges<br>**Epinions:** 75,877 nodes, 811,478 edges |
| [103] | 2018 | Generic | Detection of Sybil | **Random walk framework:** Evaluate each node trust score<br>Decomposed the network into three subgraphs: friendship, activity-following and user-activity graph | Not Available | Crawled Twitter network consists of 450,242 accounts and 222,944,310 links, which comprise 409,694 benign accounts, 40,548 Sybils and 17,581,069 friendship attack edges |
| [87] | 2018 | Generic | Detection of Sybils | Integrate advantages of random walk-based techniques and loopy belief propagation-based techniques | Not Available | **Synthesized Sybils:**<br>**Facebook:** 4,039 nodes, 88,234 edges<br>**Epinions:** 75,877 nodes, 811,478 edges<br>**Enron:** 33,696 nodes, 180,811 edges<br>**Real Sybils:**<br>**Twitter:** 41,652,230 nodes, 1,202,513,046 edges |
| [31] | 2018 | Generic | Detection of Sybils | Capture local account information in node trust scores<br>Propagate these scores through the global structure<br>Leverage edge trust scores | Incoming requests accepted ratio, outgoing requests accepted ratio and local clustering coefficient | Labelled Twitter network consists of 20M nodes and 265M edges |
| [97] | 2018 | Generic | Detection of Sybil | Find an embedding using stochastic gradient descent<br>Enable the embedding moving towards the global location as one node | Not Available | **LiveJournal - Injected Sybils:** 99K nodes and 2.2M directed links<br>**Renren - Real Sybils:** 60K users and 2.2M positive edges and 0.4M negative edges |
| [12] | 2012 | Generic | Detection of Sybil in a collaborative network | Latent community model for partitioning a graph into subnetworks | The vector of community sizes, the number of nodes in the ith community, the upper-triangular matrix of edge counts and the number of edges between community | **Irvine Community:** 1,899 nodes and 13,820 edges<br>**Wikipedia Vote:** 7115 nodes and 100,762 vote edges<br>**Gnutella Peer-to-Peer Network:** 8,717 nodes and 31,525 edges |
| [8] | 2018 | Generic | Classification of users into malicious and benign | **Machine learning:** Random forest, Adaboost and k-nearest neighbours | Weighted degree-degree centrality, weighted degree-core centrality, degree-intensity centrality, degree-coherence centrality, core-intensity centrality, weighted degree-clustering centrality and core-coherence centrality | **Twitter dataset:** FakeProject, Elezioni2013, TWT, INT<br>All four put together and provide a network of 469,504 nodes and 2,153,426 edges<br>**Facebook:** Ego-Facebook is made of 4,039 nodes and 88,234 edges |
| [3] | 2018 | Generic | Mitigation of Sybil attacks | Utilize a random walk with absorbing states for propagating legitimate labels within the graph of social network | User profile, content level and interaction network | **Twitter:** 12952 nodes, 299515 edges<br>**Facebook:** 4,039 nodes, 88234 edges<br>**WikiVote:** 7115 nodes, 103689 edges |
| [2] | 2018 | Twitter | Detection of Sybil attack | Feed-forward neural network | Profile-based features, graph-based features and content-based features | **Dataset I:** 25,510 training profiles, 13,957 tested profiles and 42,856,800 tweets related to the USA Election from mid-December 2015<br>**Datasets II:** 2,200 training profiles, 940 tested profiles and 4,152,799 tweets after the USA election |
| [4] | 2018 | Generic | Detection of Sybil attack and providing a secure communication service among users | **Key agreement protocol:** private key generator generates parameters | Not Available | **Twitter and YouTube datasets:** 10,000 nodes, with a maximum of 1000 and a minimum of 100 connected nodes |

Table 2. Existing works on sockpuppet detection techniques - verbal behaviour analysis

| Ref | Year | Social media | Goal | Technique | Features | Datasets |
|---|---|---|---|---|---|---|
| [76] | 2013 | Wikipedia | Detection of sockpuppet to link them to their corresponding puppeteer | Gather predictions from the classifier on each comment. Combine each prediction in a majority voting schema | 239 features which capture grammatical, stylistic and formatting preferences of the writers | **English Wikipedia:** 41 Sockpuppets and 36 Non-sockpuppet |
| [105] | 2011 | Online Discussion Forums | Detection of sockpuppet pairs | **Method I:** analyse the total amount of topics published by one user with the relative amount of replies from the other user **Method II:** create a keyword-based profile of the two forums, compare similarity between the two keyword profiles | Number of topics, sum of the weights of all topics has replied and number of distinct users who have replied to the topic | **Method I:** **Uwants:** 8 million postings from Jan 2009 to Dec 2009 **Method II:** **Uwants and HK discuss forums:** 8 million postings, 2257 sockpuppet pairs' out of 1000 billion account pairs from Mar 2010 to May 2010 |
| [20] | 2015 | Twitter | Detection of sockpuppet | Use computational algorithm to delete non-UTF-8 Remove hyperlinks, user mentions and hashtags Extract n-gram features Naive Bayes classifier | N-gram features | 23 authors who had posted more than 100 tweets from June 25 to August 25, 2014 |
| [42] | 2013 | Online Discussion Forums | Detection of users with multiple aliases | **String-based matching:** the matching depends on the names of alias **Stylometric matching:** the matching depends on the post writer **Time profile-based matching:** the matching depends on the posts' publishing time **Social network-based matching:** the matching depends on friend information or thread | Word length, sentence length, letters, digits punctuation and function words | **Irish web forum site:** posts from users who have written at least 60 messages in total from 2008 |

Table 3. Existing works on sockpuppet detection techniques - non-verbal behaviour analysis

| Ref | Year | Social media | Goal | Technique | Features | Datasets |
|---|---|---|---|---|---|---|
| [81] | 2014 | Generic | Detection of multiple account identity deception | **Machine learning:** Random forest, support vector machine and Adaboost | Number of total revisions since initial registration, number of total revisions for (article, user page, article discussion and user discussion page) and file uploads and images | **Wikipedia:** sampled 12723 users which roughly 48.23% were sockpuppets from February 2004 to October 2013 |
| [54] | 2017 | Online Discussion Forums | Detection of sockpuppets | Build in the manner that Wikipedia administrators do to recognise sockpuppets. Discover users that make comparable edits on the same article by considering the editing time and user's IP address | Community features, activity features and post features | **Nine online discussion forums:** 2,897,847 accounts, 62,744,175 posts and 2,129,355 discussions |
| [95] | 2018 | Generic | Detection of group sockpuppet | **Machine learning:** Support vector machine, random forest, naive Bayes, k-nearest neighbour, Bayesian network and Adaboost | Action behaviour, other accounts behaviour regard to actions of an account and characteristics of account | **English Wikipedia:** 10,000 accounts, 50% of them are blocked and 50% of them are active users |
| [94] | 2015 | Generic | Detection of fake accounts registered by the same user | **Machine learning:** Random forest, logistic regression and support vector machine. | Pattern features, basic distribution features and frequency features | **Labelled LinkedIn account data:** 260,644 accounts 153,019 fake accounts and 107,625 legitimate from December 1, 2013 to May 31, 2014. |

Table 4. Existing works on sockpuppet detection techniques - similar-orientation network

| Ref | Year | Social media | Goal | Technique | Features | Datasets |
|---|---|---|---|---|---|---|
| [58] | 2016 | Generic | Detection of Sockpuppet gang account | Random Walks<br>**Multiple community detection:** Girvan Newman, BGLL algorithm and overlap propagation algorithm | Number of comments, and time interval series of all the comments and time interval between the post time and comments | **Two master boards from Ifeng.com:**<br>**IT datasets:** 5200 accounts, 87487 comments and 198969 historical comments, 448 popular topics<br>**Social datasets:** 6522 accounts, 21323 comments and 711278 historical comments, 150 most popular topics |
| [91] | 2018 | Generic | Observing characteristics of sockpuppets | Construct for each user: interaction network graph and interest network graph<br>Subgraph similarity matching | Account activities (graph that links accounts through interactions) | **Sina Weibo user's homepage:** 2,890 sockpuppets and 48,309 ordinary users |
| [57] | 2019 | Generic | Investigation into the differences of propagation trees between sockpuppet and ordinary account | Construct propagation tree<br>**Machine learning:** Logistic regression, support vector machine, random forest and Adaboost | Propagation behaviour features | Crawled tweets from Sina Weibo from January 2017 to October 2018 |
| [106] | 2019 | Generic | Studying sockpuppets' temporal character of social networks | Construct the social graph<br>Design a weight representation method<br>Formalize sockpuppets detection as a similarity time-series analysis problem | Not Available | **Sina Weibo user's homepage:** 4,035 sockpuppets and 48,309 legitimate users, including their posts, profiles and information of the social network |
| [92] | 2018 | Facebook | Detection of multiple accounts that created by the same user | Unsupervised learning using Katz similarity<br>Semi-supervised learning using Katz similarity<br>Semi-supervised learning using Graph embedding | Not Available | Crawled from Facebook for more than five years<br>**Dataset I:** 188 accounts, 262 activities<br>**Dataset II:** 4188 accounts, 6715 activities |
| [64] | 2010 | Generic | Detection of multiple phantom gaming profile | **Classification:** Support vector machine | Phantom users' characteristics | **Fighters' Club (FC):** 2,532,779 fights, 80,174,483 support requests, 264,606 unique users, 30,990 unique installed users, 545 known phantom users, 520 known genuine users, 70,209 fights instigated by genuine users, 61,751 fights targeting genuine users, 105,704 fights instigated by phantom users, 341,389 fights targeting phantom users for two years |

Table 5. Existing works on social botnet detection techniques

| Ref | Year | Social media | Goal | Technique | Features | Datasets |
|---|---|---|---|---|---|---|
| [24] | 2014 | Generic | Studying the problem of identifying bots on Twitter from an application perspective | **Classification techniques:** Support vector machine, Adaboost, Gaussian naive Bayes, gradient boosting, random forests and extremely randomized trees | Tweet syntax, tweet semantics, user behaviour and user neighbourhood | **India Election dataset:** 550,000 Twitter accounts and 7.7 million tweets from July 15, 2013, to March 24, 2014 |
| [102] | 2018 | Twitter | Investigation of the effectiveness and advantages of exploiting a social botnet for spam distribution | **Botnet-based spam distribution:** track each account's history participating in spam distribution<br>**Digital-influence manipulation:** find sufficient honest accounts to use their actions in order to calculate digital-influence scores for other accounts. | Not Available | Built a Twitter subnet consist of 6,000 legitimate accounts and 400 social bots |
| [50] | 2018 | Twitter | Detection of fake Twitter account and bots | Neural network model on the decision values resulting from the support vector machine | Following rate, age of the account, bidirectional link ratio, average neighbours followers, average neighbours tweets, followings to median neighbours followers, API URL ratio and API ratio | **MIB dataset:**<br>**The Fake Project:** 469 volunteers accounts<br>**elezioni2013 dataset:** 1481 Twitter accounts |
| [7] | 2019 | Twitter | Studying the relationship between bots and genuine human users and identifying credulous users | **Machine learning:** Decision trees, random forest, RIPPER and neural network | User-based, Friends-based, Network-based, Temporal-based, Content-based and Sentiment-based | **Twitter Dataset I:** 754 human users, 126,000 friends, 17,000 bots<br>**Twitter Dataset II:** 377 humans, 65,000 friends, and 8,000 bots<br>**Twitter Dataset III:** 188 humans, exposing 35,000 friends and 4,000 bots |
| [17] | 2012 | Twitter | Classification of Twitter accounts into human, bot, cyborg | **Classification technique:** Random forest | Entropy, URL ratio, automated device, Bayesian spam detection, link safety and hashtag ratio | Collection of 500,000 users with 40 million tweets from Twitter for one month |
| [52] | 2018 | Twitter | Detection of bots at the tweet level | **Classification tasks:**<br>**Account-level bot detection:** synthetic minority oversampling technique (SMOTE)<br>**Tweet-level bot detection:** Long short-term memory | **Account- level bot detection:** Statuses Count, followers count, geo enables, friends count, favorites count, default profile, listed count, profile uses background image, verified and protected<br>**Tweet-level bot detection:** Retweet count, reply count, favorite count, hashtags number, URLs number and mentions number | **Genuine accounts:** 3474 accounts, 8,377,522 tweets from 2011<br>**Social spambots 1:** 991 accounts 1,610,176 tweets from 2012<br>**Social spambots 2:** 3457 accounts 428,542 tweets from 2014<br>**Social spambots 3**: 464 accounts, 1,418,626 tweets from 2011 |

Table 6. Existing works on other fake profile detection techniques

| Ref | Year | Social media | Goal | Technique | Features | Datasets |
|---|---|---|---|---|---|---|
| [84] | 2018 | Generic | Evaluation of using the engineered features that detect bot account to detect fake account created by human | **Machine learning:** Random forest, Adaboost, support vector machine | Account age, account has a duplicate profile, ratio of friends-to-followers, account has a profile image, name and description, description contains URL and username length | **Twitter:** 200 million tweets from 223 796 accounts from 2006 and 2017 |
| [15] | 2018 | Twitter | Differentiate between fake accounts and real accounts | Analyse RFDs between fake, real and verified account | 15 attributes for individual accounts | **Twitter APIs:** 9019 accounts, 3949 Verified, 1757 Real, 3313 Fake from September 2018 |
| [34] | 2015 | Twitter | Understanding the characteristics of fake account creation | Map-reducing<br>Pattern recognition | ID, followers count, friends count, verified, created at, description, location, updated, profile image URL and screen name | Crawled user profiles on Twitter for three-month period in late 2013<br>62 million raw user profiles |
| [55] | 2018 | Facebook | Identifying potential fake users based on their activities and profile information | User gives permission to the app to access their information<br>The app calculates the trust between the user and his Facebook friends. | Number of mutual friends, is family, age group, average likes and average comments | Not Available |
| [86] | 2010 | Twitter | Identification of suspicious users | **Machine learning:** Neural network, decision tree, support vector machine and naive Bayes | Graph-based features and content-based features | **Twitter:** 500 Twitter user accounts are manually labelled into two classes: non-spam and spam |
| [107] | 2012 | Generic | Detection of spammers | Supervised Matrix Factorization method with social regularization | Latent features | Select 30,000 active normal accounts, 700 spammer accounts from Renren.com by using community detection algorithm [? ] from 2 December 2011 to 8 December 2011 |
| [74] | 2016 | Twitter | Analysing of behaviour of Twitter users tweeting pornographic content | **Classification techniques:** Random forest, Bayes network, logistic regression, J48 classifier and Adaboost | Graph-based features and content-based features | Crawled from Twitter from 27 April 2015 to 8 May 2015<br>**Genuine accounts:** 8522 accounts with their 17,04,400 tweets<br>**Pornographic accounts:** 10,300 accounts with their 20,60,000 tweets |
| [8] | 2014 | Twitter | Detection of spammers | **Machine learning:** Support vector machine | Content and behaviour features | Crawled from Twitter from August 2009<br>54 million accounts, 1.9 billion links and almost 1.8 billion tweets |
| [5] | 2014 | Twitter | Detection of user genders deception | **Classification techniques:** hybrid naive Bayes and decision-tree | Different profile characteristics (first name, username and layout colours) | Crawled user profiles on Twitter from January 2014 to February 2014 194,292 profiles, of which 104,535 males and 89,757 females |
| [79] | 2017 | Generic | Prevention of deceptive account form participating in online sub-communities | Create a view of sub-community's network.<br>The network does not include isolated nodes. Use centrality metrics to generate a profile for the position of each node in a network and describe how critical a node is | Not Available | Ban list provided by the giftcardexchange subreddit from September 2014 to December 2015 419 banned accounts, 419 legitimate accounts |

Table 7. Existing works on compromised account detection techniques

| Ref | Year | Social media | Goal | Technique | Features | Datasets |
|---|---|---|---|---|---|---|
| [88] | 2018 | Generic | Detection of identity theft | Joint probabilistic generative model based on Bayes network Tensor decomposition-based method | Check-in location in offline behaviour space and user generated content in online behaviour space | **Foursquare:** 31493 users, 143923 venues and 267319 check-ins **Yelp:** 80,592 users, 42,051 venues and 491,393 check-ins |
| [48] | 2018 | Generic | Detection of compromised account using authorship verification | Classification and statistical analysis | N-grams, Bag of words (BOW), stylometric and folksonomy | **Twitter:** 1,47,909 users with each user having at most 500 tweets |
| [70] | 2018 | Generic | Detection of compromised account | Uni-gram language and KL-divergence measure | Textual features | **Twitter corpus:** 467 million posts from 20 million users for 7 months |
| [75] | 2018 | Twitter | Detection of different types of spammers including compromised accounts | **Machine learning:** Naive Bayes, logistic regression, J48, random forest, Adaboost | User-based features, content-based features and trust-based features | Crawled from Twitter for 3 months 1,00,000 accounts with their 20 million tweets, 8522 users with their 17,04,400 tweets, 476 spam accounts with their 95,200 tweets, 10,298 pornographic storytellers and 285 follower market merchants |
| [14] | 2014 | Facebook and Instagram | Designing and implementing a malicious account detection system | **Clustering technique:** Hadoop | User activity | Facebook and Instagram from August 2013 |
| [85] | 2016 | Generic | Detection of identity theft | Transform the connection time information to a feature Train a binary support vector machine classifier Estimate the false alarm and detection probabilities that reflect its performance | Connection time | **WOSN dataset - Facebook wall posts:** 46,952 users |

Table 8. Existing works on other detection techniques of identity theft

| Ref | Year | Social media | Goal | Technique | Features | Datasets |
|---|---|---|---|---|---|---|
| [18] | 2012 | Facebook | Detection of impersonating a real person | Find anomalies by comparing the profile network structure to the typical social network graph structure for the population | Average degree of the nodes in the social network graph and number of singleton friends in the social network graph | **Facebook:** 80 profiles |
| [36] | 2014 | Generic | Protecting users from identity theft attack | **Experiment 1:** compare the similarities between user accounts among online social media sites. **Experiment 2:** compare the friend network similarity | Number of common friends and number of account's friend | **Experiment 1:** questionnaires - 200 samples from internet users **Experiment 2:** questionnaires - volunteer's and her 22 friends' contacts list |
| [100] | 2017 | News articles | Understanding identity thieves and fraudsters behaviours | Text mining techniques | Personally identifiable Information (PII) | Google News, NewYork Times 3500 identity theft-related news stories from February 2014 to April 2014 |

Table 9. Existing works on identity cloning detection techniques

| Ref | Year | Social media | Goal | Technique | Features | Datasets |
|---|---|---|---|---|---|---|
| [51] | 2011 | Generic | Detection of cloned profile | Similarity scores between the collected profiles and the real profile | Profile information | **LinkedIn:** 1,120 public profiles |
| [23] | 2014 | Generic | Detection of cloned profile | Extract information from user's profile<br>Extract information from profiles having same name as user<br>Calculate similarity index for all profiles | Name, workplace, Birthdate education, profile photo, places lived, gender and number of friends/connections | Facebook, LinkedIn, Google+<br>10 subjects |
| [41] | 2011 | Generic | Detection of suspicious identities and then validating them | Basic Profile Similarity (BPS) and Multiple-Faked Identities Profile Similarity (MFIPS) | Number of similar public attributes and the number of common friends | **Facebook:** 63731 users, 1634115 friend links, 3629 faked identities |
| [44] | 2017 | Generic | Matching user profile across multiple social media | Classifier based on FuzzySim and friend similarity to detect colluders in friend requests | Name, profile photo, workplace, education, places lived, Birthdate and gender | **Synthetic dataset:** Facebook and Google+<br>2000 people Profiles |

Table 10. Domains of identity deception detection techniques

| **Domains** | **Detection Techniques** | | | | | | |
|---|---|---|---|---|---|---|---|
| | **Fake Profile** | | | | **Identity Theft** | | **Identity Cloning** |
| | Sybil | Sockpuppets | Social Botnet | Other | Compromised Account | Other | |
| **Generic** | [3] [4] [8] [12] [31] [40] [87] [97] [103] | [58] [64] [81] [92] [91] [94] [95] [106] | [24] | [79] [84] [107] | [36] [85] | [48] [70] [88] | [23] [41] [44] [51] |
| **Twitter** | [2] | [20] | [7] [50] [52] | [5] [8] [15] [17] [34] [74] [86] [102] | [75] | | |
| **Facebook** | | [92] | | [14] [55] | | [18] | |
| **Discussion forums** | | [42] [54] [105] | | | | | |
| **Wikipedia** | | [76] | | | | | |
| **Instagram** | | | | [14] | | | |
| **News articles** | | | | | | [100] | |

Table 11. Identity deception detection techniques

| Detection Techniques | | | | | | | |
|---|---|---|---|---|---|---|---|
| | Fake Profile | | | | Identity Theft | | Identity Cloning |
| | Sybil | Sockpuppets | Social Botnet | Other | Compromised Account | Other | |
| Machine learning-based | [2] [3] [4] [8] | | [7] [17] | [5] [8] [74] [84] [107] | [14] [75] [85] | | |
| Graph-based | [31] [40] [87] [97] [103] | | | [79] [86] | | [18] [36] | [44] |
| Similar-orientation network | | [58] [64] [91] [92] [106] | | | | | |
| Verbal behaviour analysis | | [20] [42] [76] [105] | | | | | |
| Non-verbal behaviour analysis | | [54] [81] [94] [95] | | | | | |
| User Profile-Based | | | | | | | [23] [41] [51] |
| Text mining-based | | | [24] [102] | | | | |
| Key management-based | [4] | | | | | | |
| Deep learning-based | | | [52] | | | | |
| Behaviour-based | | | | | | [88] | |
| Textual-based | | | | | | [48] [70] | |
| Data mining-based | | | | | | | [100] |
| Other | | | | [15] [34] [55] | | | |

Table 12. Features of identity deception detection techniques 1

| **Features** | **Detection Techniques** | | | | | | |
|---|---|---|---|---|---|---|---|
| | | **Fake Profile** | | | **Identity Theft** | | **Identity Cloning** |
| | Sybil | Sockpuppets | Social Botnet | Other | Compromised Account | Other | |
| **Content feature** | | | | | | | |
| Number of posts | [2] [3] | [54] [58] [92] [105] | [7] | [8] [15] [55] | [75] | | |
| Number of characters | [2] | [54] | [7] | [8] | [48] | | |
| Fraction of punctuations | [2] | [54] | [7] | | [48] | | |
| Number of syllables | [2] | [54] | | | [48] | | |
| Readability metrics | | [54] | | | | | |
| Diversity of pages modified | | [95] | | | | | |
| Number of hashtags | [2] | | [7] [17] [24] | [86] | [48] | | |
| Number of user mentions | [2] [3] | | [7] [17] [24] [52] | [8] [86] | [48] | | |
| Number of links | | | [24] [52] | [8] [15] [34] [55] [74] [86] | [75] | | |
| Number of special characters | [2] | | [24] | [8] | [48] | | |
| Number of retweets | [3] | | [52] | [74] | [48] | | |
| Sending duplicate tweet repeatedly | | | | [74] | [75] | | |
| Number of malicious links | | | | | [75] | | |
| Number of replies | [3] | | | | | | |
| Number of emotions | [2] | | | | | | |
| N-gram feature | | [105] | | | [48] | | |
| **User profile feature** | | | | | | | |
| Number of distinct users | [3] | [105] | | | | | |
| Number of followers | [2] [3] | | [7] [52] | [8] [74] [84] [86] [15] [34] | [75] | | |
| Reputation | | | | [74] [86] | [75] | | |
| Characterization of screen names | [2] | | | [15] [34] [74] [84] | | | |
| Characterization of description | [2] | | | [5] [15] [34] [74] [84] | | | |
| Background color | | | | [5] [15] | | | |
| Location | [2] | | | [15] [34] | | | |
| Verified | [2] | | | [34] | | | |
| Profile image | [2] | | | [15] [84] | | | |
| Number of friends | [2] [3] | | | [55] | | | |
| URL in description | [2] | | | [84] | | | |
| Common account | | | | | [75] | | |
| Profile information | | | | | | | [23] [41] [44] [51] |
| **Time feature** | | | | | | | |
| Time between posts | [2] | [54] [58] | [7] | | [75] | | |
| Tenure time | | [54] | | | | | |
| Delay between account's registration and first action | | [95] | | | | | |
| Time between the post time and comments | [2] | [58] | | | | | |
| Account age | [2] | | | [8] [55] [84] | [75] | | |
| Median of the duration of all connections within the day | | | | | [85] | | |
| Overall duration of connections | | | | | [85] | | |
| Mean duration averaged over the longest eight daily connections | | | | | [85] | | |
| Number of hours with at least one connection | | | | | [85] | | |

Table 13. Features of identity deception detection techniques 2

| Features | Detection Techniques | | | | | | |
|---|---|---|---|---|---|---|---|
| | Fake Profile | | | | Identity Theft | | Identity Cloning |
| | Sybil | Sockpuppets | Social Botnet | Other | Compromised Account | Other | |
| **Graph feature** | | | | | | | |
| Interaction Graph | | [91] | | | | | |
| Core-coherence centrality | [8] | | | | | | |
| Degree of the nodes | | | | | | [18] | |
| Number of singleton friends | | | | | | [18] | |
| The vector of community sizes | [12] | | | | | | |
| Weighted degree-core centrality | [8] | | | | | | |
| The number of nodes | [12] | | | | | | |
| The upper-triangular matrix of edge counts | [12] | | | | | | |
| Core-intensity centrality | [8] | | | | | | |
| The number of edges | [12] | | | | | | |
| Weighted degree-clustering centrality | [8] | | | | | | |
| Degree-intensity centrality | [8] | | | | | | |
| Degree-coherence centrality | [8] | | | | | | |
| Weighted random walk | [31] | | | | | | |
| Weighted loopy belief propagation | [31] | | | | | | |
| **Distribution feature** | | | | | | | |
| **Numerical feature** | | | | | | | |
| Min | | [94] | | | [70] | | |
| Max | | [94] | | | [70] | | |
| Quartiles | | [94] | | | | | |
| Mean | | [94] | | | [70] | | |
| Variance | | [94] | | | | | |
| **Categorical feature** | | | | | | | |
| Number of distinct feature values | | [94] | | | | | |
| Percentage of values that are unique | | [94] | | | | | |
| Percentage of null values | | [94] | | | | | |
| Percentage of values belonging to the mode | | [94] | | | | | |
| **Structure feature** | | | | | | | |
| Number of total revisions | | [81] | | | | | |
| File uploads | | [81] | | | | | |
| Images | | [81] | | | | | |
| Average topic sentiment | | | [24] | | | | |
| **Community feature** | | | | | | | |
| Whether account is blocked | | [54] | | | | | |
| Fraction of reported | | [54] [95] | | | | | |
| Fraction of deleted posts | | [54] | | | | | |
| **Propagation tree feature** | | | | | | | |
| Average depth of propagation tree | | [92] | | | | | |
| Average size of propagation tree | | [92] | | | | | |
| Average index of type of posts | | [92] | | | | | |
| Average number of identical account in tree | | [92] | | | | | |
| Average Depth of only one 1-hop repost of original post | | [92] | | | | | |
| Average number of children of propagation tree | | [92] | | | | | |
| Average maximum depth and width | | [92] | | | | | |
| Average interval between interactions | | [92] | | | | | |

Table 14. Evaluation metrics of identity deception detection techniques

| **Evaluation metrics** | **Detection Techniques** | | | | | | |
|---|---|---|---|---|---|---|---|
| | | **Fake Profile** | | | **Identity Theft** | | **Identity Cloning** |
| | Sybil | Sockpuppets | Social Botnet | Other | Compromised Account | Other | |
| Accuracy | [2] [31] | [42] [58] [64] [76] [81] [91] [92] [105] [106] | [7] [17] [50] [52] | [5] [74] [79] [84] [95] | [48] [70] [75] | | [41] |
| Precision | [97] | [20] [57] [76] [81] [91] [92] [95] [106] | [52] [102] | [8] [74] [79] [84] [86] [107] | [14] [48] [70] [75] [88] | | [44] |
| Recall | [97] | [20] [57] [76] [81] [91] [92] [106] | [24] [52] | [8] [74] [79] [84] [86] [107] | [48] [70] [75] [88] | | [44] |
| False Positive Rate | [12] [40] | [57] [64] [81] [91] [95] [106] | [24] [102] | [34] [74] [79] | [14] [48] [75] [88] | | |
| F-measure | | [20] [57] [76] [81] [91] [92] [95] [106] | [52] | [79] [84] [86] [107] | [48] [70] | | |
| False Negative Rate | [12] [40] | [64] [81] [95] | | [74] | [48] [75] | | |
| Area Under The Curve (AUC) | [31] [87] [103] | [54] [95] | [52] | [84] | [88] | | |
| Matthews Correlation | | [81] [95] | | [79] | | | |
| Receiver Operating Characteristic (ROC) | [1] | | [52] | | | | |
| Coefficient of Variance (CV) | [95] | | | | [48] | | |
| False Rejection Rate | | | | | [48] | | |
| False Acceptance Rate (FAR) | | | | | [48] | | |

Table 15. Datasets of identity deception detection techniques

| **Datasets** | **Detection Techniques** | | | | | | |
|---|---|---|---|---|---|---|---|
| | **Fake Profile** | | | | **Identity Theft** | | **Identity Cloning** |
| | Sybil | Sockpuppets | Social Botnet | Other | Compromised Account | Other | |
| Twitter | [40] [87] | | [7] [17] [24] [50] [52] | [5] [8] [15] [34] [74] [84] [86] | [48] [70] [75] | | |
| Facebook | [3] [40] [8] [87] | [64] [92] | | | [14] | [18] | [41] [44] |
| Wikipedia | [3] [12] | [76] [81] [95] | | | | | |
| Enron | [40] [87] | | | | | | |
| Epinions | [40] [87] | | | | | | |
| LinkedIn | | [94] | | | | | [51] |
| Renren | [97] | | | [107] | | | |
| Irvine | [12] | | | | | | |
| Gnutella | [12] | | | | | | |
| LiveJournal | [97] | | | | | | |
| Uwants and HK | | [105] | | | | | |
| Ifeng.com | | [58] | | | | | |
| Sina Weibo | | [92] | | | | | |
| Reddit | | | | [79] | | | |
| Instagram | | | | [14] | | | |
| Foursquare | | | | | [88] | | |
| Yelp | | | | | [88] | | |
| Google+ | | | | | | | [44] |
| Google News, and NewYork Times | | | | | | [100] | |
